# Supplementary material for: Synthesizing Linked Data Under Cardinality and Integrity Constraints
Source: arXiv:2103.14435 source file (2021-03-26)
Supplement: Supplementary file 1 [file appendix.tex]

\section{Appendix}
The set $S_{CC}$ of cardinality constraints used with only the predicates that apply to $R_1$ columns (that were used with $Ten$ and/or $Area$ predicates):
\begin{itemize}
    \item $Age\in[18, 114], Rel$=Owner, $Sex$=M.
    \item $Age\in[18, 114], Rel$=Spouse, $Sex$=F.
    \item $Age\in[21, 114], Rel$=Spouse, $Sex$=F.
    \item $Age\in[21, 64], Rel$=Spouse, $Sex$=F.
    \item $Age\in[18, 39], Rel$=Spouse, $Sex$=F.
    \item $Age\in[18, 85], Rel$=Spouse, $Sex$=F.
    \item $Age\in[40, 85], Rel$=Spouse, $Sex$=F.
    \item $Age\in[0, 10], Rel$=Biological child; similarly for $Age\in [6, 10]$ and $[2, 5]$.
    \item $Age\in[3, 5], Rel$=Biological child, $Sex$=M.
    \item $Age\in[11, 18], Rel$=Biological child; similarly for $Age\in [11, 13], [14, 18], [19, 30]$ and $[22, 30]$.
    \item $Age\in[65, 114], Rel$=Father or Mother.
    \item $Age\in[40, 85], Rel$=Father or Mother, $Sex$=M.
    \item $Age\in[40, 85], Rel$=Father or Mother, $Sex$=F.
    \item $Age\in[65, 114], Rel$=Father or Mother, $Sex$=F.
    \item $Age\in[15, 85], Rel$=Housemate or Roommate.
    \item $Age\in[15, 85], Rel$=Housemate or Roommate, $Sex$=M.
    \item $Age\in[15, 85], Rel$=Housemate or Roommate, $Sex$=F.
    \item $Age\in[18, 30], Rel$=Grandchild, $Sex$=M.
    \item $Age\in[0, 39], Rel$=Grandchild, $Sex$=F.
    \item $Age\in[22, 39], Rel$=Grandchild, $Sex$=F.
    \item $Age\in[18, 30], Rel$=Grandchild, $Sex$=F.
    \item $Age\in[18, 114], Rel$=Unmarried partner, $Sex$=F.
    \item $Age\in[0, 30], Rel$=Stepson or stepdaughter.
    \item $Age\in[0, 21], Rel$=Stepson or stepdaughter.
    \item $Age\in[19, 39], Rel$=Adopted child.
    \item $Age\in[25, 39], Rel$=Adopted child, $Sex$=F.
    \item $Age\in[31, 39], Rel$=Adopted child, $Sex$=F.
\end{itemize}

The set $S_{DC}$ of denial constraints used:
\begin{enumerate}
    \item No biological, adoptive or step- child can have an age outside of $[A-69, A-12]$ when the householder is male.
    \item No biological, adoptive or step- child can have an age outside of $[A-50, A-12]$ when the householder is female.
    \item No spouse or unmarried partner can have an age outside of $[A-50, A+50]$.
    \item No sibling can have an age outside of $[A-35, A+35]$.
    \item No parent or parent-in-law can have an age outside of $[A+12, A+115]$.
    \item No grandchild can have an age outside of $[A-115, A-30]$.
    \item No son-/daughter-in-law can have an age outside of $[A-69, A-1]$.
    \item No foster-child can have an age outside of $[A-69, A-12]$.
    \item No two householders can share a household.
    \item If $A<30$, then the number of grandchildren and son-/daughter-in-law in the household must be $0$.
    \item If $A>94$, then the number of parent and parent-in-law in the household must be $0$.
    \item No two spouses or unmarried partners can share a household.
\end{enumerate}
